# Supplementary material for: Distant RF field sensing with a passive Rydberg-atomic transducer
Source: arXiv:2306.15215 source file (2023-09-20)
Supplement: Supplementary file 1 [file supplementary.pdf]

# Distant RF field sensing with a passive Rydberg-atomic transducer: Supplementary Material

## SENSOR PERFORMANCE FOR OFF-RESONANT RF FIELDS

Figure S1 presents the SNR of the sensor for an off-resonant two-photon EIT case at a distance of 10 m between the base station and the sensing unit. For the measurement, the probe laser was stabilized to the D<sub>2</sub>-line and the coupling laser frequency was scanned over the 49D<sub>5/2</sub> and 49D<sub>3/2</sub> Rydberg frequencies. An RF field with carrier frequencies between 16 and 20 GHz and with  $f_{\text{AM}} = 60$  kHz was applied to the antenna. The retrieved AM signals dependent on the carrier frequency and the coupling frequency detuning for four different powers of the RF carrier field are shown in Fig. S1. As expected, independent of the RF carrier power, the sensor has the highest SNR for a resonant EIT scheme (zero coupling detuning). With increasing RF carrier power, the sensor becomes sensitive to off-resonant RF frequencies in accordance with the observation in Fig. 2. Moreover, as shown in Fig. S1(c) and (d), for large RF carrier powers the  $m_j$ -dependent ( $m_j = 1/2, 3/2, 5/2$ ) AC Stark shifts [1] start to resolve, resulting in sensitive areas for coupling detunings left of the zero detuning line. Additionally, in Fig. S1(c) and (d) we observe that the signal disappears at  $\sim 17$  GHz. We attribute this to a cancellation of the AC Stark shifts of the 49D<sub>5/2</sub> state caused by the two adjacent states 50P<sub>3/2</sub> and 48F<sub>7/2</sub>, which contribute a counteracting shift [2].

## REFERENCES

1. J. Hu, H. Li, R. Song, *et al.*, “Continuously tunable radio frequency electrometry with Rydberg atoms,” *Appl. Phys. Lett.* **121**, 014002 (2022).
2. D. H. Meyer, Z. A. Castillo, K. C. Cox, and P. D. Kunz, “Assessment of Rydberg atoms for wideband electric field sensing,” *J. Phys. B: At. Mol. Opt. Phys.* **53**, 034001 (2020).

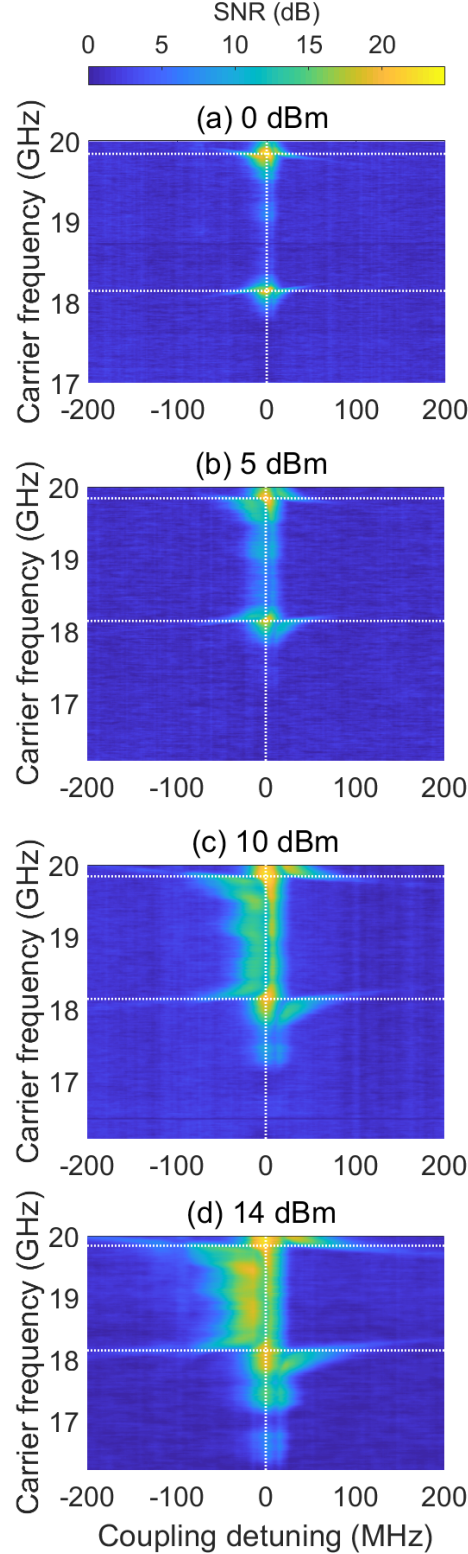

**Fig. S1.** SNR dependent on the frequency of the coupling field and RF carrier frequency for four different RF carrier powers (a to d). An amplitude modulation at 60 kHz with a modulation depth of 95 % is applied to the RF carrier field. For each RF power, the carrier frequency is changed in 20 MHz steps between 16 and 20 GHz. The SNR is measured using a spectrum analyzer in zero span mode with a resolution bandwidth of 1 kHz. For the frequency calibration of the x-axis, we make use of the transmission signal through a high-finesse cavity and the 20 MHz sidebands used for the Pound-Drever-Hall technique.
